# Supplementary material for: Online Collaborative Resource Allocation and Task Offloading for Multi-access Edge Computing
Source: arXiv:2501.02952 source file (2025-01-06)
Supplement: Supplementary file 1 [file Appendices.tex]

\documentclass[10pt,journal,compsoc]{IEEEtran}
%documentclass[journal]{IEEEtran}
\usepackage{graphicx}
\usepackage{epstopdf}
\usepackage{multirow}
\usepackage{amssymb}
\usepackage{amsmath}
\usepackage{color}
\usepackage[linesnumbered,algoruled,boxed,lined]{algorithm2e}
\usepackage{amssymb}
\usepackage{array}
\usepackage{subfigure} 
\usepackage{cases}
\usepackage{comment}
\definecolor{b}{rgb}{0.0, 0, 1}
\definecolor{k}{rgb}{0, 0, 0}
\usepackage{xr}
\makeatletter
\newcommand*{\addFileDependency}[1]{
  \typeout{(#1)}
  \@addtofilelist{#1}
  \IfFileExists{#1}{}{\typeout{No file #1.}}
}
\makeatother

\newcommand*{\myexternaldocument}[1]{
    \externaldocument{#1}
    \addFileDependency{#1.tex}
    \addFileDependency{#1.aux}
}

%%% 主文件名称
\myexternaldocument{manuscript}

\setlength{\abovedisplayskip}{8pt}
\setlength{\belowdisplayskip}{8pt}
\setlength{\abovedisplayshortskip}{8pt}
\setlength{\belowdisplayshortskip}{8pt}
\newenvironment{sequation}{\begin{equation}\small}{\end{equation}}

\ifCLASSOPTIONcompsoc
  % IEEE Computer Society needs nocompress option
  % requires cite.sty v4.0 or later (November 2003)
  \usepackage[nocompress]{cite}
\else
  % normal IEEE
  \usepackage{cite}
\fi

\definecolor{color}{rgb}{0.0, 0, 0}

\ifCLASSINFOpdf
\else
\fi

% correct bad hyphenation here
\hyphenation{op-tical net-works semi-conduc-tor}

\begin{document}

\title{Appendices \\ \vspace{23pt} \Large{\textit{Online Collaborative Resource Allocation and Task Offloading for Multi-access Edge Computing}}}

\markboth{Appendices}%
{Shell \MakeLowercase{\textit{et al.}}: Bare Demo of IEEEtran.cls for Computer Society Journals}

\maketitle 

\IEEEpeerreviewmaketitle

\appendices

%
% proof Upper bound of Lyapunov drift-plus-penalty function 
%
\section{Proof of Theorem \ref{the_bound_drift}}
\label{app_the_bound_drift}

\par On the one hand, we present the bounds related to the task queues $Q_{m}^{\text{E}}(t)$ and $Q_{m}^{\text{C}}$. First, for any non-negative real number $\vartheta_1 \geq 0$, $\vartheta_2  \geq 0$, $\vartheta_3 \geq 0$, we can deduce the inequality as follows:
\begin{sequation}
\label{eq_inequality1}
\begin{aligned}
&(\max \{\vartheta_1-\vartheta_2 , 0\}+\vartheta_3)^2  \\
&\leq (\max \{\vartheta_1-\vartheta_2 , 0\})^2+ (\vartheta_3)^2+2\max \{\vartheta_1-\vartheta_2 , 0\}\vartheta_3\\
&\leq (\vartheta_1-\vartheta_2)^2+ (\vartheta_3)^2+2\vartheta_1\vartheta_3\\
&= \vartheta_1^2+\vartheta_2 ^2+\vartheta_3^2+2 \vartheta_1(\vartheta_3-\vartheta_2).
\end{aligned}
\end{sequation}

\par Then, based on the inequality \eqref{eq_inequality1} of the main paper, we can deduce the inequality by squaring Eq. \eqref{eq_deadline_QL} of the main paper as follows:
\begin{sequation}
\label{eq_inequality2}
\begin{aligned}
{[Q_m^{\text{E}}(t+1)]^2 \leq } & {[Q_m^{\text{E}}(t)]^2+\big[A_m^{\text{E}}(t)\big]^2+\big[\frac{f_{m}\delta}{\rho}\big]^2 } \\
& +2 Q_m^{\text{E}}(t)\big[A_m^{\text{E}}(t)-\frac{f_{m}\delta}{\rho}\big] .
\end{aligned}
\end{sequation}

\par Furthermore, we can obtain the inequality from \eqref{eq_inequality2} as
\begin{sequation}
\begin{aligned}
& \frac{1}{2}\big\{[Q_m^{\text{E}}(t+1)]^2-[Q_m^{\text{E}}(t)]^2\big\} \\
& \leq \frac{1}{2}\Big\{[A_m^{\text{E}}(t)]^2+\big[\frac{f_{m}\delta}{\rho}\big]^2+2 Q_m^{\text{E}}(t)\big[A_m^{\text{E}}(t)-\frac{f_{m}\delta}{\rho}\big]\Big\}.
\end{aligned}
\end{sequation}

\par Similarly, based on \eqref{eq_inequality1} and  \eqref{eq_deadline_QO} of the main paper, we can derive the bounds associated with $Q_m^{\text{O}(t)}$ as follows:
\begin{sequation}
\begin{aligned}
& \frac{1}{2}\big\{[Q_m^{\text{C}}(t+1)]^2-[Q_m^{\text{C}}(t)]^2\big\} \\
&\leq \frac{1}{2}\big\{[A_m^{\text{C}}(t)]^2+[r_{m}^{c}\delta]^2+2 Q_m^{\text{C}}(t)[A_m^{\text{C}}(t)-r_{m}^{c}]\big\}.
\end{aligned}
\end{sequation}

\par On the other hand, we present the bounds associated with the virtual queues $Z_{m}^{\text{E}}(t)$ and $Z_{m}^{\text{C}}$. First, for any non-negative real numbers $\vartheta_1 \geq 0$, $\vartheta_2  \geq 0$, $\vartheta_3 \geq 0$, we can deduce the inequality as 
\begin{sequation}
\label{eq_inequality3}
\begin{aligned}
(\max\{\vartheta_1-\vartheta_2 +\vartheta_3,0\})^2 & \leq (\max \{\vartheta_1-\vartheta_2 , 0\}+\vartheta_3)^2 \\
& \leq \vartheta_1^2+\vartheta_2 ^2+\vartheta_3^2+2 \vartheta_1(\vartheta_3-\vartheta_2).
\end{aligned}
\end{sequation}

\par Moreover, based on \eqref{eq_inequality3}, we can obtain the inequality by squaring Eq. \eqref{eq_deadline_QO} of the main paper as follows:
\begin{sequation}
\label{eq_inequality4}
\begin{aligned}
{[Z_{m}^{\text{E}}(t+1)]^2 \leq } & {[Z_{m}^{\text{E}}(t)]^2+\big[\frac{Q_{m}^{\text{E}}(t)}{\tilde{A}_{m}^{\text{E}}|(t)}\big]^2+[\bar{D}_{m}^{\text{E}}]^2 } \\
& +2 Z_{m}^{\text{E}}(t)\Big[\frac{Q_{m}^{\text{E}}(t)}{\tilde{A}_{m}^{\text{E}}|(t)}-\bar{D}_{m }^{\text{L}}\Big] .
\end{aligned}
\end{sequation}

\par Besides, we can deduce the inequality from \eqref{eq_inequality4} as follows:
\begin{sequation}
\label{eq_inequality5}
\begin{aligned}
 \frac{1}{2}&\big\{[Z_{m}^{\text{E}}(t+1)]^2-[Z_{m}^{\text{E}}(t)]^2\big\}
\leq \frac{1}{2}\Big\{\big[\frac{Q_m^L(t)}{\tilde{A}_m^L(t)}\big]^2\\
&+(D_{m, \max }^L)^2+2 Z_{m}^{\text{E}}(t)\big[\frac{Q_m^L(t)}{\tilde{A}_m^L(t)}-D_{m, \max }^L\big]\Big\} .
\end{aligned}
\end{sequation}

\par Similarly, based on \eqref{eq_inequality3} and \eqref{eq_virtual_O} of the main paper, we can derive the bounds associated with $Z_m^{\text{O}(t)}$ as follows:
\begin{sequation}
\begin{aligned}
 \frac{1}{2}&\big\{[Z_{m}^{\text{C}}(t+1)]^2- [Z_{m}^{\text{C}}(t)]^2\big\}
\leq \frac{1}{2}\Big\{\big[\frac{Q_m^{\text{C}}(t)}{\tilde{A}_m^{\text{C}}(t)}\big]^2 \\
&\phantom{vvvvv}+(D_{m, \max }^{\text{C}})^2+2 Z_{m}^{\text{C}}(t)\big[\frac{Q_m^{\text{C}}(t)}{\tilde{A}_m^{\text{C}}(t)}-D_{m, \max }^{\text{C}}\big]\Big\} .
\end{aligned}
\end{sequation}

%
% proof Problem $\mathbf{\bar{P}^{\prime\prime\prime}.1}$ 
%
\section{Proof of Theorem \ref{lem_P1_convex}}
\label{app_lem_P1_convex}
\par First, objective function \eqref{RA1} of the main paper can be re-expressed as
\begin{sequation}
    J(\hat{\mathcal{X}}, \mathcal{A}) = \sum_{u \in \mathcal{U}_m^{\text{O}}} f_u(a_u^m(t)) + \phi,
\end{sequation}

\noindent where 
\begin{sequation}
   \label{eq_fuau}
    f_u(a_u^m(t)) = \frac{V \beta_u(t)}{a_u^m(t) B_m}.
\end{sequation}

\par Secondly, the second derivative of \eqref{eq_fuau} in terms of $a_u^m(t)$ can be calculated as
\begin{sequation}
    f_u^{\prime\prime}(a_u^m(t)) = \frac{2V \beta_u(t)}{a_u^{3m}(t) B_m}.
\end{sequation}

\noindent Since \( a_u^m(t) > 0 \) and \( V, \beta_u(t), B_m > 0 \), we have \( f_u^{\prime\prime}(a_u^m(t)) > 0 \), confirming that \( f_u(a_u^m(t)) \) is a convex function. Therefore, the objective function is also convex because the sum of convex functions is also convex~\cite{boyd2004convex}. 

\par Finally, constraints \eqref{RA_a} and \eqref{RA_b} of the main paper are linear inequalities. As a result, problem $\mathbf{\bar{P}^{\prime\prime\prime}.1}$ is convex.

%
% proof of optimal communication resource allocation
%
\section{Proof of Theorem \ref{theo_opt_resource}}
\label{app_theo_opt_resource}

\par First, the Lagrangian function of problem $\mathbf{\bar{P}^{\prime\prime\prime}.1}$ can be given as~\cite{LiuFZ2023} 

\vspace{-0.8em}
{\small
{
\begin{align}
\mathcal{L}(J(\mathcal{X}, \mathcal{A}), \lambda)&=\sum_{u \in \mathcal U_m^{\text{O}}}\frac{ V \beta _k(t)}{a_{u}^{m}(t)B_m}+\phi+\lambda \big( \sum_{k \in \mathcal U_m^{\text{O}}} a_{u}^{m}(t) - 1\big),
\end{align}
}
}

\noindent where $\lambda$ represents the Lagrange multiplier. Then, the karush-kuhn-tucker (KKT) conditions can be obtained as 

\vspace{-0.8em}
{\small
\begin{subequations}
\label{eq_KKT}
\begin{alignat}{1}
        &\frac{\partial \mathcal{L}(J(\hat{\mathcal{X}}, \mathcal{A})}{\partial  a_{u}^{m}(t)}=0, \, \forall u\in \mathcal{U}_m^{\text{O}}\label{eq_KKT_stat}\\
        &a_{u}^{m}(t)\geq 0, \forall u\in \mathcal{U}_m^{\text{O}},\label{eq_KKT_fea1}\\
        &\sum_{u \in \mathcal U_m^{\text{O}}} a_{u}^{m}(t) \leq 1, \label{eq_KKT_fea2} \\
        &\lambda \ge 0, \label{eq_KKT_dual} \\
        &\lambda \big( \sum_{k \in \mathcal U_m^{\text{O}}} a_{u}^{m}(t) - 1\big)= 0, \label{eq_KKT_comple} 
\end{alignat}
\end{subequations}
}

\noindent where \eqref{eq_KKT_stat} represents the stationarity condition, \eqref{eq_KKT_fea1} and \eqref{eq_KKT_fea2} indicate primal feasibility, \eqref{eq_KKT_dual} ensures dual feasibility, and \eqref{eq_KKT_comple} is the complementary slackness condition.

\par Based on Theorem \ref{lem_P1_convex}, $\mathbf{\bar{P}^{\prime\prime\prime}.1}$ is a convex optimization problem. Accordingly, the solution that satisfies the KKT conditions is the optimal solution of problem $\mathbf{\bar{P}^{\prime\prime\prime}.1}$ \cite{dutta2013optimality}. Therefore, the optimal communication resource allocation can be obtained by solving the KKT conditions.

%
% proof of P2
%
\section{Proof of Theorem \ref{lem_P2_INLP}}
\label{app_lem_P2_INLP}

\par Problem $\mathbf{\bar{P}^{\prime\prime\prime}.2}$ involves only binary variables. Moreover, the objective function contains nonlinear terms, as the decision variables are as the denominator of fractional expressions. Consequently, problem $\mathbf{\bar{P}^{\prime\prime\prime}.2}$ is an integer nonlinear programming (INLP) problem, which is NP-hard.

%
% proof of P21
%
\section{Proof of Theorem \ref{lem_P21_ILP}}
\label{app_lem_P21_INLP}

\par Problem $\mathbf{\bar{P}^{\prime\prime\prime}.2.1}$ Problem $\mathbf{\bar{P}^{\prime\prime\prime}.2.1}$ involves only binary variables, and the objective function is linear with respect to the decision variables. Consequently, problem $\mathbf{\bar{P}^{\prime\prime\prime}.2.1}$ is an integer linear programming (ILP) problem, which is NP-hard.

%
%  at least one of the two fractional solutions
%
\section{Proof of Theorem \ref{lem_round_1}}
\label{app_lem_round_1}
 
\par We consider the different cases for the parameters $\iota_1$ and $\iota_2$ in the rounding process.

\begin{itemize}
    \item Case 1: $\iota_1 = 1 - x_{u1}^{m \rightarrow c}$ and $\iota_2 = x_{u1}^{m \rightarrow c}$. If Eq. \eqref{eq_frac_to_int_1} of the main paper is executed, $(x_{u1}^{m \rightarrow c})^{\prime} = x_{u1}^{m \rightarrow c} - \iota_2 = 0$. Similarly, if Eq. \eqref{eq_frac_to_int_2} of the main paper is executed, $(x_{u1}^{m \rightarrow c})^{\prime}=x_{u1}^{m \rightarrow c}+\iota_1=1$. Thus, one of the solutions is rounded to 0.

    \item Case 2: $\iota_1 = 1 - x_{u1}^{m \rightarrow c}$ and $\iota_2 = \frac{\varpi _{u2}^{m \rightarrow c}}{\varpi _{u1}^{m \rightarrow c}}(1 - x_{u2}^{m \rightarrow c})$. If Eq. \eqref{eq_frac_to_int_1} of the main paper is executed, it can be deduced that $(x_{u2}^{m \rightarrow c})^{\prime} = x_{u2}^{m \rightarrow c} + \frac{\varpi _{u1}^{m \rightarrow c}}{\varpi _{u2}^{m \rightarrow c}}  \frac{\varpi _{u2}^{m \rightarrow c}}{\varpi _{u1}^{m \rightarrow c}} (1 - x_{u2}^{m \rightarrow c}) = 1$. If Eq. \eqref{eq_frac_to_int_2} of the main paper is executed, it can be obtained that $(x_{u1}^{m \rightarrow c})^{\prime} = x_{u1}^{m \rightarrow c} + \iota_1 = 0$. Therefore, one of the solutions is rounded to 0.

    \item Case 3: $\iota_1 = \frac{\varpi _{u2}^{m \rightarrow c}}{\varpi _{u1}^{m \rightarrow c}}x_{u2}^{m \rightarrow c}$ and $\iota_2 = x_{u1}^{m \rightarrow c}$. If Eq. \eqref{eq_frac_to_int_1} of the main paper is executed, we can obtain 
    $(x_{u1}^{m \rightarrow c})^{\prime} = x_{u1}^{m \rightarrow c} - \iota_2 = 0$. If Eq. \eqref{eq_frac_to_int_2} of the main paper is executed, it can be deduced that $(x_{u2}^{m \rightarrow c})^{\prime} = x_{u2}^{m \rightarrow c} - \frac{\varpi _{u1}^{m \rightarrow c}}{\varpi _{u2}^{m \rightarrow c}}  \iota_1 = x_{u2}^{m \rightarrow c} - \frac{\varpi _{u1}^{m \rightarrow c}}{\varpi _{u2}^{m \rightarrow c}}  \frac{\varpi _{u2}^{m \rightarrow c}}{\varpi _{u1}^{m \rightarrow c}}x_{u2}^{m \rightarrow c} = 0$. Accordingly, at least one of the solutions is rounded to either 0 or 1.

    \item Case 4: $\iota_1 = \frac{\varpi _{u2}^{m \rightarrow c}}{\varpi _{u1}^{m \rightarrow c}}x_{u2}^{m \rightarrow c}$ and $\iota_2 = \frac{\varpi _{u2}^{m \rightarrow c}}{\varpi _{u1}^{m \rightarrow c}}(1 - x_{u2}^{m \rightarrow c})$. If Eq. \eqref{eq_frac_to_int_1} of the main paper is executed, it can be obtained that $(x_{u2}^{m \rightarrow c})^{\prime}=x_{u2}^{m \rightarrow c}+\frac{\varpi _{u1}^{m \rightarrow c}}{\varpi _{u2}^{m \rightarrow c}}\iota_2=x_{u2}^{m \rightarrow c}+\frac{\varpi _{u1}^{m \rightarrow c}}{\varpi _{u2}^{m \rightarrow c}}\frac{\varpi _{u2}^{m \rightarrow c}}{\varpi _{u1}^{m \rightarrow c}}(1 - x_{u2}^{m \rightarrow c})=1$. If Eq. \eqref{eq_frac_to_int_2} of the main paper is executed, we can obtain 
    $(x_{u2}^{m \rightarrow c})^{\prime} = x_{u2}^{m \rightarrow c} + \iota_1 = x_{u2}^{m \rightarrow c} + \frac{\varpi _{u2}^{m \rightarrow c}}{\varpi _{u1}^{m \rightarrow c}}x_{u2}^{m \rightarrow c} = 1$. Therefore, one of the solutions will be rounded to 0 or 1.
\end{itemize}

\par In all three cases, after each rounding action, at least one fractional solution is rounded to either 0 or 1.

%
%  whether updating the fractional solutions
%
\section{Proof of Theorem \ref{lem_round_2}}
\label{app_lem_round_2}

\par If the fractional solutions are transformed into integral solutions according to Eq. \eqref{eq_frac_to_int_1} of the main paper, it can be obtained that $
(x_{u1}^{m \rightarrow c})^{\prime} = x_{u1}^{m \rightarrow c} - \iota_2,
(x_{u2}^{m \rightarrow c})^{\prime} = x_{u2}^{m \rightarrow c} + \frac{\varpi_{u1}^{m \rightarrow c}}{\varpi_{u2}^{m \rightarrow c}} \iota_2
$. We can further deduced that

\vspace{-0.8em}
{\small
\begin{align}
&(x_{u1}^{m \rightarrow c})^{\prime}  \varpi_{u1}^{m \rightarrow c} + (x_{u2}^{m \rightarrow c})^{\prime}  \varpi_{u2}^{m \rightarrow c} \notag\\ 
&= (x_{u1}^{m \rightarrow c} - \iota_2)  \varpi_{u1}^{m \rightarrow c} + \big(x_{u2}^{m \rightarrow c} + \frac{\varpi_{u1}^{m \rightarrow c}}{\varpi_{u2}^{m \rightarrow c}} \iota_2\big) \varpi_{u2}^{m \rightarrow c} \notag\\
&= x_{u1}^{m \rightarrow c}  \varpi_{u1}^{m \rightarrow c} + x_{u2}^{m \rightarrow c}  \varpi_{u2}^{m \rightarrow c}.
\end{align}}

If the fractional solutions are transformed into integral solutions according to Eq. \eqref{eq_frac_to_int_2} of the main paper, we have $(x_{u1}^{m \rightarrow c})^{\prime} = x_{u1}^{m \rightarrow c} + \iota_1,
(x_{u2}^{m \rightarrow c})^{\prime}= x_{u2}^{m \rightarrow c} - \frac{\varpi_{u1}^{m \rightarrow c}}{\varpi_{u2}^{m \rightarrow c}} \iota_1$.  We can further deduced that

\vspace{-0.8em}
{\small
\begin{align}
&(x_{u1}^{m \rightarrow c})^{\prime} \varpi_{u1}^{m \rightarrow c} + (x_{u2}^{m \rightarrow c})^{\prime} \varpi_{u2}^{m \rightarrow c} \notag\\ 
&=(x_{u1}^{m \rightarrow c} + \iota_1)\varpi_{u1}^{m \rightarrow c} + \big(x_{u2}^{m \rightarrow c} - \frac{\varpi_{u1}^{m \rightarrow c}}{\varpi_{u2}^{m \rightarrow c}} \iota_1\big)  \varpi_{u2}^{m \rightarrow c} \notag\\
&= x_{u1}^{m \rightarrow c}  \varpi_{u1}^{m \rightarrow c} + x_{u2}^{m \rightarrow c} \varpi_{u2}^{m \rightarrow c}.
\end{align}}

\par In conclusion, it is guaranteed that the relationship 
\(
x_{u1}^{m \rightarrow c} \varpi_{u1}^{m \rightarrow c} + x_{u2}^{m \rightarrow c} \varpi_{u2}^{m \rightarrow c} = (x_{u1}^{m \rightarrow c})^{\prime} \varpi_{u1}^{m \rightarrow c} + (x_{u2}^{m \rightarrow c})^{\prime}\varpi_{u2}^{m \rightarrow c}
\) 
holds true in a rounding action, regardless of whether the fractional solutions are updated according to Eq. \eqref{eq_frac_to_int_1} or Eq. \eqref{eq_frac_to_int_2} of the main paper.

%
%  complexity
%
\section{Proof of Theorem \ref{the_complexty}}
\label{app_the_complexty}

\par The OJCTA consists of two stages in each time slot. In the first stage, the offloading decision is determined by using Algorithm \ref{al_two_stage}. In the second stage, the communication resource allocation decision is derived from the close-form solution in Eq. \eqref{eq_theo_opt_resource} of the main paper. Consequently, the computational complexity is primarily determined by the first stage, i.e., Algorithm \ref{al_two_stage}. Assuming that the number of outer iterations in Algorithm \ref{al_two_stage} is $L$, each iteration involves executing Algorithms \ref{algo_matching} and \ref{algo_cvx_rounding} sequentially. For Algorithm \ref{algo_matching}, the computational complexity mainly stems from the swap matching process, resulting in a complexity of $\mathcal{O}(U^2)$. For Algorithm \ref{algo_cvx_rounding}, the computational complexity is $\mathcal{O}(U^3)$ according to \cite{Wang2022Deep}. Thus, the overall complexity of OJCTA is $\mathcal{O}(LU^3)$.
%
%  gap
%
\section{Proof of Theorem \ref{the_gap}}
\label{app_the_gap}

\par According to~\cite{2010Neely}, for any $\lambda_1,\lambda_2,\lambda_3,\lambda_4>0$, there is a stationary and randomized policy $\backepsilon$ for problem $\mathbf{P^{\prime\prime}}$ which makes the following inequalities hold.

\vspace{-0.8em}
{\small
\begin{subequations}
    \label{eq_the_lemma_bound}
    \begin{alignat}{1}
          &\mathbb{E}\left\{ C( \mathcal{A}^\backepsilon(t), \mathcal{X}^\backepsilon(t) ) \mid \Theta(t)\right\}\le C^{\text{opt}}+\max\{\lambda_1,\lambda_2,\lambda_3,\lambda_4\}, \\
          &\mathbb{E}\left\{ A_m^{\text{E}}(t)-\frac{f_m\delta}{\rho} \mid \Theta(t),\mathcal{A}^\backepsilon(t), \mathcal{X}^\backepsilon(t)\right\}\le \lambda_1,\\
         &\mathbb{E}\big\{ A_{m}^{\text{C}}(t)-r_{m}^c\delta \mid \Theta(t),\mathcal{A}^\backepsilon(t), \mathcal{X}^\backepsilon(t)\big\}\le \lambda_2,\\
        &\mathbb{E}\big\{ \frac{Q_{m}^{\text{E}}(t)}{\tilde{A}_{m}^{L}(t)}-\bar{D}_{m}^{\text{E}} \mid \Theta(t),\mathcal{A}^\backepsilon(t), \mathcal{X}^\backepsilon(t)\big\}\le \lambda_3,\\
        &\mathbb{E}\big\{ \frac{Q_{m}^{\text{E}}(t)}{\tilde{A}_{m}^{L}(t)}-\bar{D}_{m}^{\text{E}} \mid \Theta(t),\mathcal{A}^\backepsilon(t), \mathcal{X}^\backepsilon(t)\big\}\le \lambda_4.
    \end{alignat}
\end{subequations}}

\par  Therefore, by substituting the policy $\backepsilon$ into Eq. \eqref{eq_drift_bound}, we can obtain the inequalities as
\begin{sequation}
\begin{aligned}
&\Delta(\Theta(t))+ V\mathbb{E}\{ C( \mathcal{A}(t), \mathcal{X}(t)) \mid \Theta(t)\} \\
&\le B + V\mathbb{E}\big\{ C\left( \mathcal{A}^\backepsilon(t), \mathcal{X}^\backepsilon(t) \right) \mid \Theta(t)\big\} \\
&\quad +\sum_{m=1}^{M}  \bigg(Q_{m}^{\text{E}}(t) \mathbb{E}\big\{A_m^{\text{E}}(t)-\frac{f_m\delta}{\rho} \mid \Theta(t),\mathcal{A}^\backepsilon(t), \mathcal{X}^\backepsilon(t)\big\} \\
&\quad + Q_{m}^{\text{C}}(t) \mathbb{E}\big\{A_{m}^{\text{C}}(t)-r_{m}^c\delta \mid \Theta(t),\mathcal{A}^\backepsilon(t), \mathcal{X}^\backepsilon(t)\big\} \\
&\quad + Z_{m}^{E}(t) \mathbb{E}\big\{\frac{Q_{m}^{\text{E}}(t)}{\tilde{A}_{m}^{L}(t)}-\bar{D}_{m}^{\text{E}} \mid \Theta(t),\mathcal{A}^\backepsilon(t), \mathcal{X}^\backepsilon(t)\big\} \\
&\quad + Z_{m}^{\text{C}}(t) \mathbb{E}\big\{\frac{Q_{m}^{\text{C}}(t)}{\tilde{A}_{m}^{C}(t)}-\bar{D}_{m}^{\text{C}} \mid \Theta(t),\mathcal{A}^\backepsilon(t), \mathcal{X}^\backepsilon(t)\big\} \bigg)\\
&\le B +V\big(C^{\text{opt}}+\max\{\lambda_1,\lambda_2,\lambda_3,\lambda_4\}\big)\\
&\quad +\sum_{m=1}^{M}\big(Q_{m}^{\text{E}}(t)\lambda_1+Q_{m}^{\text{C}}(t)\lambda_2+Z_{m}^{E}(t)\lambda_3+Z_{m}^{C}(t)\lambda_4\big)
\end{aligned}
\end{sequation}

\par By letting $\lambda_1,\lambda_2,\lambda_3,\lambda_4$ approach zero, summing the inequality over all time slots, and then dividing each side by $VT$, we can obtain the ineuality as follows:
\begin{sequation}
\begin{aligned}
\frac{1}{T} \mathbb{E}[L(\Theta(T))&-L(\Theta(0))]+ \frac{1}{T}\sum_{t=1}^{T}\mathbb{E}\left\{ C\left( \mathcal{A}(t), \mathcal{X}(t) \right) \mid \Theta(t)\right\} \\
&\le \frac{B}{V}+C^{\text{opt}}.
\end{aligned}
\end{sequation}

\noindent Since $L(\Theta(T))=0$ and $\lim _{T \rightarrow \infty} \frac{1}{T}L(\Theta(T)) =0$, we can derive \eqref{eq_teh_bound} of the main paper.

\bibliographystyle{IEEEtran}
\bibliography{references.bib}
\end{document}
